# Supplementary material for: Maximum Weighted Loss Discrepancy
Source: arXiv:1906.03518 source file (2019-06-08)
Supplement: Supplementary file 1 [file appendix_experiments.tex]

\begin{figure}
	\centering
	\begin{subfigure}[b]{\textwidth}
		\includegraphics[width=0.9\textwidth]{images/new/worst_group_german.png}
		\label{fig:gull}
	\end{subfigure}
	\begin{subfigure}[b]{\textwidth}
		\includegraphics[width=0.9\textwidth]{images/new/worst_group_adult.png}
		\label{fig:tiger}
	\end{subfigure}
	
	\begin{subfigure}[b]{\textwidth}
		\includegraphics[width=0.9\textwidth]{images/new/worst_group_candc.png}
		\label{fig:mouse}
	\end{subfigure}
	\caption{Top row: german dataset, middle row: adult dataset, last row: c\&c dataset}\label{fig:animals}
\end{figure}

\begin{figure}
	\centering
	\begin{subfigure}[b]{\textwidth}
		\includegraphics[width=0.9\textwidth]{images/new/showing_gerrymandering_german.png}
		\label{fig:gull}
	\end{subfigure}
	\begin{subfigure}[b]{\textwidth}
		\includegraphics[width=0.9\textwidth]{images/new/showing_gerrymandering_adult.png}
		\label{fig:tiger}
	\end{subfigure}
	
	\begin{subfigure}[b]{\textwidth}
		\includegraphics[width=0.9\textwidth]{images/new/showing_gerrymandering_candc.png}
		\label{fig:mouse}
	\end{subfigure}
	\caption{Top row: german dataset, middle row: adult dataset, last row: c\&c dataset}\label{fig:animals}
\end{figure}

\begin{figure}
	\centering
	\begin{subfigure}[b]{\textwidth}
		\includegraphics[width=0.9\textwidth]{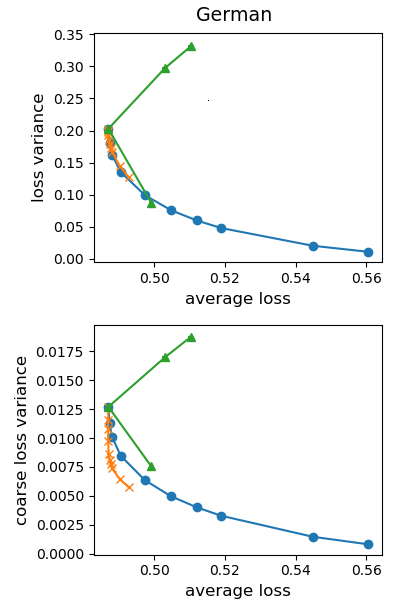}
		\label{fig:gull}
	\end{subfigure}
	\begin{subfigure}[b]{\textwidth}
		\includegraphics[width=0.9\textwidth]{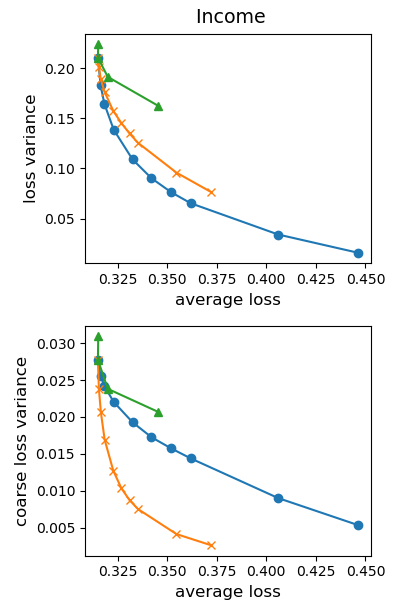}
		\label{fig:tiger}
	\end{subfigure}
	
	\begin{subfigure}[b]{\textwidth}
		\includegraphics[width=0.9\textwidth]{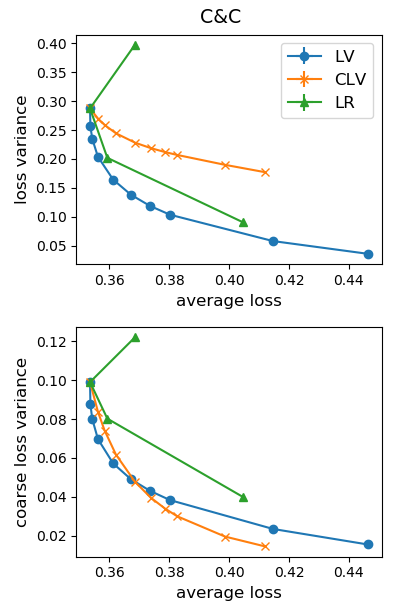}
		\label{fig:mouse}
	\end{subfigure}
	\caption{Top row: german dataset, middle row: adult dataset, last row: c\&c dataset}\label{fig:animals}
\end{figure}

\begin{figure}
	\centering
	\begin{subfigure}[b]{\textwidth}
		\includegraphics[width=0.9\textwidth]{images/new/individual_visualization_german.png}
		\label{fig:gull}
	\end{subfigure}
	\begin{subfigure}[b]{\textwidth}
		\includegraphics[width=0.9\textwidth]{images/new/individual_visualization_adult.png}
		\label{fig:tiger}
	\end{subfigure}
	
	\begin{subfigure}[b]{\textwidth}
		\includegraphics[width=0.9\textwidth]{images/new/individual_visualization_candc.png}
		\label{fig:mouse}
	\end{subfigure}
	\caption{Top row: german dataset, middle row: adult dataset, last row: c\&c dataset}\label{fig:animals}
\end{figure}

\begin{figure}
	\centering
	\begin{subfigure}[b]{\textwidth}
		\includegraphics[width=0.9\textwidth]{images/new/group_visualization_german.png}
		\label{fig:gull}
	\end{subfigure}
	\begin{subfigure}[b]{\textwidth}
		\includegraphics[width=0.9\textwidth]{images/new/group_visualization_adult.png}
		\label{fig:tiger}
	\end{subfigure}
	
	\begin{subfigure}[b]{\textwidth}
		\includegraphics[width=0.9\textwidth]{images/new/group_visualization_candc.png}
		\label{fig:mouse}
	\end{subfigure}
	\caption{Top row: german dataset, middle row: adult dataset, last row: c\&c dataset}\label{fig:animals}
\end{figure}

\begin{figure}
	\centering
	\begin{subfigure}[b]{\textwidth}
		\includegraphics[width=0.9\textwidth]{images/new/subgroup_visualization_german.png}
		\label{fig:gull}
	\end{subfigure}
	\begin{subfigure}[b]{\textwidth}
		\includegraphics[width=0.9\textwidth]{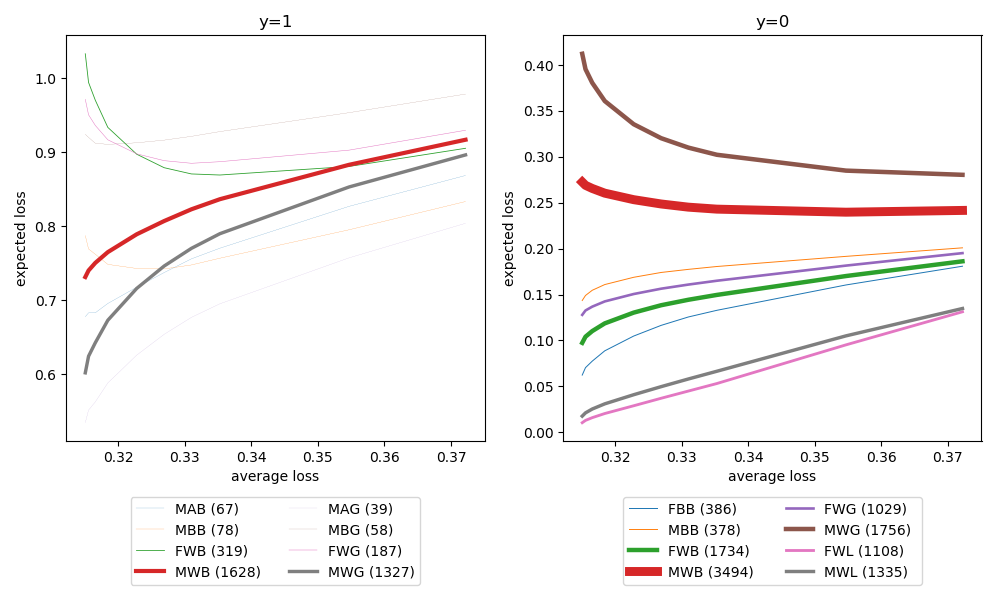}
		\label{fig:tiger}
	\end{subfigure}
	
	\begin{subfigure}[b]{\textwidth}
		\includegraphics[width=0.9\textwidth]{images/new/subgroup_visualization_candc.png}
		\label{fig:mouse}
	\end{subfigure}
	\caption{Top row: german dataset, middle row: adult dataset, last row: c\&c dataset}\label{fig:animals}
\end{figure}

\begin{figure}
	\centering
	\begin{subfigure}[b]{\textwidth}
		\includegraphics[width=0.9\textwidth]{images/new/comparison5_german.png}
		\label{fig:gull}
	\end{subfigure}
	\begin{subfigure}[b]{\textwidth}
		\includegraphics[width=0.9\textwidth]{images/new/comparison5_adult.png}
		\label{fig:tiger}
	\end{subfigure}
	
	\begin{subfigure}[b]{\textwidth}
		\includegraphics[width=0.9\textwidth]{images/new/comparison5_candc.png}
		\label{fig:mouse}
	\end{subfigure}
	\caption{Top row: german dataset, middle row: adult dataset, last row: c\&c dataset}\label{fig:animals}
\end{figure}

\begin{figure}
	\centering
	\begin{subfigure}[b]{\textwidth}
		\includegraphics[width=0.9\textwidth]{images/new/comparison20_german.png}
		\label{fig:gull}
	\end{subfigure}
	\begin{subfigure}[b]{\textwidth}
		\includegraphics[width=0.9\textwidth]{images/new/comparison20_adult.png}
		\label{fig:tiger}
	\end{subfigure}
	
	\begin{subfigure}[b]{\textwidth}
		\includegraphics[width=0.9\textwidth]{images/new/comparison20_candc.png}
		\label{fig:mouse}
	\end{subfigure}
	\caption{Top row: german dataset, middle row: adult dataset, last row: c\&c dataset}\label{fig:animals}
\end{figure}
