# Supplementary material for: Maximum Weighted Loss Discrepancy
Source: arXiv:1906.03518 source file (2019-06-08)
Supplement: Supplementary file 2 [file appendix_figures2.tex]

-\section{Appendix B}
-\subsection{Loss variance effects on groups}
-\begin{table*}
	\centering
	\scalebox{0.8}{
	\begin{tabular}{llll}
		\toprule
		\bf Loss variance & \bf Formula & \bf Protected groups & \bf Examples on Income dataset\\ \midrule
			Group  & $\max_i \var [\ell \mid A_i]$ & $\sG^*_{A_i}$: Sensitive coarse groups (groups defined on $A_i$) & women\\
			Subgroup  & $\var [\E [\ell \mid A]]$& $\sG^*_A$: Sensitive fine groups (groups defined on $A$) & non white women\\
			Individual & $\var [\ell]$& 
			$\sG^*$: All groups (groups defined on $\sX$)& non white married women\\
			\bottomrule
	\end{tabular}}
	\caption{\label{tab:different_regularizers} Different loss variances and the groups that can be protected by bounding them.}
\end{table*}
-\input{group_visualization}
-For better understanding group regularizer we plot the trade-off between expected loss of sensitive groups and the average loss \reffig{group_regularizer} (Remember we compute this trade-off by increasing $\lambda$ in \refeqn{ermReg} )
-As shown, groups such as Male, White, Greater and 25 over predicted to having high paid jobs; therefore they have higher loss when $y=0$ (they really have low paid jobs); and lower loss when $y=1$.
-On the other hand, groups such as: Female, Less than 25, Black, have high loss when $y=1$; which means they over predicted to have low paid jobs and having low loss when $y=0$.
-As we increase $\lambda$\refeqn{ermReg} these groups get forced to have similar losses  when they have similar labels.
-
-\reffig{subgroup_regularizer} shows the loss of different sensitive subgroups and effect of subgroup regularizer on them.
-Looking at sensitive subgroups instead of groups, makes it more clear which subgroups are discriminated the most and also it prevents gerrymandering. 
-For example, from this diagram we can understand white male greater than 45 are the most privileged group. 
-%Or we can see while for white people being greater than 45 is better but for Asian being between 25-45 is better. 
-
-
-
-\input{worst_group_overtime}
-Recall, group-unfairness $U(\sG)$ (\refdef{group_unfairness}) is the worst-case difference in the loss of a group in $\sG$ and population loss.
-We define the conditional version of it as follows:
-\begin{align}
-\label{eqn:group-unfairness-conditional}
-\nonumber U(\sG \mid y=b) \eqdef& \max \limits_{g \in \sG} \E[g\mid y=b]  \\
-&\Big( \E[ \ell \mid g=1, y=b] -  \E[\ell \mid y=b] \Big)^2.
-\end{align}
-In \refprop{groupToVar} we showed it can get upper bounded by loss variance.
-Here as we condition on $y$, \reftab{group_unfairness_loss_variance} shows the relation between for different loss variances.
-\reffig{worst_group} shows the relation of $U(g)$ and variance for $y=1$ and Income dataset.
-We found these diagrams for other datasets and for $y=0$ similar as this one.
-(\refprop{finding_g_efficiently} shows how we find the most unfair group efficiently).
-
-
-\input{ind_sub_comparison}
-Finally for better understanding of difference between individual regularizer and subgroup regularizer, we pick the 10\% of individuals with highest loss (with label $0$) and we track their loss as we regularize both subgroup and individual regularizers.
-\reffig{ind_sub_dif_income}(left) shows the expected loss of this group in Income dataset.
-As we saw previously, in this dataset subgroup regularizer works well.
-therefore, its trade-of is a bit worse than individual regularizer but it is good on a group that is not among groups that is protecting.
-On the other hand, In \reffig{ind_sub_dif_candc}(left), subgroup regularizer did not work very well; therefore causes this group to have even higher loss as increase the amount of regularizer.
-The red dashed line show the provided guarantee that individual regularizer provide, according to \refprop{varToGroup}
-
-
-We pick the top 10 sensitive subgroups with the highest loss and track their loss as we apply subgroup/individual regularizer.
-In income dataset these subgroup are \fk{}
-In C\&C dataset these subgroup are \fk{}.
-\reffig{ind_sub_dif_income}(right) shows the difference between individual and subgroup regularizer for this group in Income dataset.
-Individual regularizer try to bring the expected loss of any group down therefore, in comparison to subgroup regularizer it does not improve loss of this group (as it is already have low loss). 
-\reffig{ind_sub_dif_candc} (right) shows in C\&C dataset, individual regularizer work almost as good as subgroup regularizer even for sensitive fine groups.
-
-
-
-\subsection{Unfairness variance relation}
-
-\input{worst_group}
-In \refsec{framework} we showed loss variance is a good surrogate to use instead of group with the maximum weighted difference loss.
-Let $U(g)$ shows the unfairness incurs on group $g$
-Formally, $U(g) = \E [g]\p{\E[\ell\mid g=1] - \E [\ell]}^2$.
-In \refprop{groupToVar}, we showed:
-$
-\max_{g\in\sG^*} U(g) \le \var [\ell] \le C\max_{g\in\sG^*} U(g)
-$.
-Where $C=2+4\ln\p{\frac{L}{\max \sqrt{U(g)}}}$, and $L$ is the maximum loss on individuals.
-Similar bounds holds for group variance and subgroup variance (See \reftab{variance_unfairness_relation}).
-\reffig{worst_group_bounds} shows these three values on real datasets.
-In \refsec{loss_variance_regularizer} we show that as we regularize loss variance the gap between $\max U(g)$ and $\var[\ell]$ shrinks.
-
-\fk{Should I bring some reasoning why these bound do not look good? e.g., Note that $L \ge 12$ which result to an upper bound of $\frac{L^2}{4} = 36$  on variance.
	-	This is right now is then bound with 4? should I change the proof or no one care about the bound anyway!}
-
-
-\fk {add how to compute $\max \E(g)(\E(\ell \mid g))...$ and why this is not np-complete, while $\max \E [\ell \mid g]$ is. }
-
-\subsection{Datasets statistics}
-
-\begin{figure}
	-	\begin{subfigure}[b]{0.25\textwidth}
		-		\includegraphics[width=\textwidth]{images/new/candc_statistics}
		-		\caption{C\&C}
		-		\end{subfigure}%
	-		\begin{subfigure}[b]{0.25\textwidth}
		-			\includegraphics[width=\textwidth]{images/new/german_statistics}
		-			\caption{German}
		-		\end{subfigure}%
	-		\begin{subfigure}[b]{0.25\textwidth}
		-			\includegraphics[width=\textwidth]{images/new/adult_statistics}
		-			\caption{Income}
		-		\end{subfigure}%
	-		\begin{subfigure}[b]{0.25\textwidth}
		-			\includegraphics[width=\textwidth]{images/new/compas_5_statistics}
		-			\caption{COMPAS}
		-		\end{subfigure}
	-\end{figure}
-
-\subsection{Comparisons}
-
-\begin{figure}
	-	\begin{subfigure}[b]{0.45\textwidth}
		-		\includegraphics[height=\textwidth]{images/new/com_zafar.png}
		-	\end{subfigure}
	-	\begin{subfigure}[b]{0.45\textwidth}
		-		\includegraphics[height=\textwidth]{images/new/group_visualization_group_01.png}
		-	\end{subfigure}
	-	\begin{subfigure}[b]{\textwidth}
		-		\includegraphics[width=\textwidth]{images/new/mis_result.png}
		-	\end{subfigure}
	-	\caption{ comparison to \cite{zafar2017fairness}}
	-\end{figure}
-
-\subsection{0-1 losses}
